# Supplementary material for: On Provable Backdoor Defense in Collaborative Learning
Source: arXiv:2101.08177 source file (2021-01-19)
Supplement: Supplementary file 1 [file c_additional_results.tex]

\section{Additional results}

Here we provide some additional examples of optimal BCC codes for reference.
We perform exhaustive search to obtain all possible codes for a certain $(k,r,n)$ and then remove those codes that are equivalent up to row and column permutations.
% There is no known polynomial time algorithms of finding these codes.
\begin{figure}[H]
    \centering
    \includegraphics[width=\textwidth]{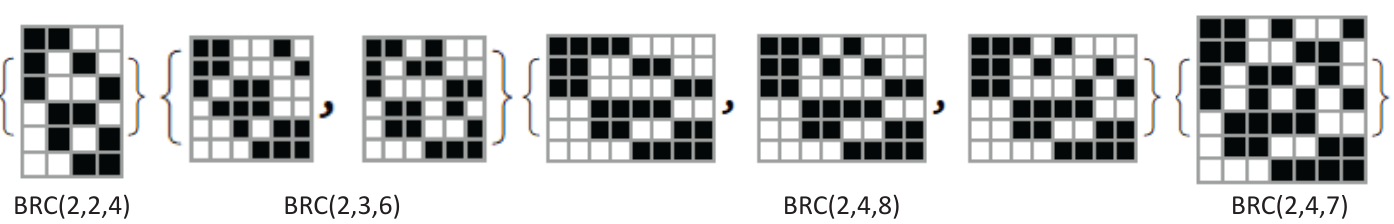}
    \caption{Optimal BRC codes obtained from exhaustive search.}
    \label{fig:codes}
\end{figure}
